# Supplementary material for: ProEvent: An Event-centric Benchmark for Proactive Agents
Source: arXiv:2607.17701 source file (2026-07-20)
Supplement: Supplementary file 1 [file Appendix_B.tex]

\section{Effects of real-world chat complexities}
\label{appendix_b}

We supplement the complete results of different models under varying numbers of negotiation turns, concurrent chats, and various noise.

\begin{table*}[h]
    \setlength{\tabcolsep}{2.5pt} % 稍微缩小列间距以适应增加的列
    \centering
    \small
    \begin{tabular}{l ccc ccc cccccccc}
        \toprule
        \multirow{3}{*}{\textbf{Models}} & \multicolumn{3}{c}{\textbf{Negotiation Turns}} & \multicolumn{3}{c}{\textbf{Multi-chat Concurrency}} & \multicolumn{8}{c}{\textbf{Noise}} \\
        \cmidrule(lr){2-4} \cmidrule(lr){5-7} \cmidrule(lr){8-15}
        & \multirow{2}{*}{T=3} & \multirow{2}{*}{T=5} & \multirow{2}{*}{T=7} & \multirow{2}{*}{N=1} & \multirow{2}{*}{N=3} & \multirow{2}{*}{N=5} & \multicolumn{2}{c}{w/o} & \multicolumn{2}{c}{w/ OT} & \multicolumn{2}{c}{w/ UE} & \multicolumn{2}{c}{w/ FA} \\
        \cmidrule(lr){8-9} \cmidrule(lr){10-11} \cmidrule(lr){12-13} \cmidrule(lr){14-15}
        & & & & & & & R & P & R & P & R & P & R & P \\
        \midrule
        DeepSeek-V3.2 & 46.5\% & 34.2\% & 27.6\% & 50.0\% & 44.4\% & 30.0\% & 53.2\% & 58.3\% & 58.9\% & 64.7\% & 53.2\% & 46.7\% & 54.4\% & 19.9\% \\
        DeepSeek-R1 & 70.3\% & 57.6\% & 56.3\% & 78.2\% & 64.5\% & 56.4\% & 67.1\% & 72.6\% & 60.8\% & 69.1\% & 53.2\% & 54.5\% & 50.6\% & 19.5\% \\
        GPT-o5.1 & \textbf{76.4\%} & \textbf{68.7\%} & \textbf{68.5\%} & \textbf{83.4\%} & \textbf{71.6\%} & \textbf{68.6\%} & 70.9\% & 76.7\% & 69.6\% & 76.4\% & 64.6\% & 73.9\% & 60.8\% & 19.8\% \\
        \midrule
        Direct & 46.5\% & 34.2\% & 27.6\% & 50.0\% & 44.4\% & 30.0\% & 53.2\% & 58.3\% & 58.9\% & 64.7\% & 53.2\% & 46.7\% & 54.4\% & 19.9\% \\
        Proactive & 45.9\% & 35.3\% & 28.5\% & 48.3\% & 43.2\% & 32.8\% & 51.9\% & 55.4\% & 61.4\% & 68.5\% & 49.4\% & 34.8\% & 49.4\% & 17.3\% \\
        ProCoT & 63.8\% & 55.1\% & 51.8\% & 53.6\% & 46.6\% & 44.6\% & 63.3\% & 72.5\% & 65.2\% & 75.8\% & 59.5\% & 65.3\% & 63.3\% & 23.7\% \\
        \bottomrule
    \end{tabular}
    \caption{}
    \label{tab:negotiation_results_extended}
\end{table*}
